# Supplementary material for: On Generalization of Adversarial Imitation Learning and Beyond
Source: arXiv:2106.10424 source file (2022-02-11)
Supplement: Supplementary file 1 [file offline.tex]

\section{Missing Proofs}

\subsection{Episodic Markov Decision Process}

In this part, we briefly introduce the episodic Markov decision process. We remark that episodic MDP is introduced to facilitate analysis since the horizon is finite. 

An episodic Markov decision process (MDP) can be described by the tuple $\gM = (\gS, \gA, \gP, r, p_0, H)$. Here $\gS$ and $\gA$ are the state and action space, respectively. $H$ is the planning horizon\footnote{$H$ corresponds to the effective horizon $1/(1-\gamma)$ in the infinite-horizon discounted MDP.}, $p_0$ is the initial state distribution, and $r: \gS \times \gA \rar [0, 1]$ is the reward function. Different from the infinite-horizon discounted MDP in \cref{sec:background}, transition function $\gP = \{p_1, \cdots, p_{H}\}$ is non-stationary. That is, $p_h(s_{h+1}|s_h, a_h)$ determines the probability of transiting to state $s_{h+1}$ conditioned on state $s_h$ and action $a_h$ in time step $h$, for $h \in [H]$\footnote{$[x]$ denotes the set of integers from $1$ to $x$.}. Since the optimal policy is not stationary, we need to consider the  non-stationary policy $\pi = \lb \pi_1, \cdots, \pi_h \rb$, where $\pi_h: \gS \rar \Delta(\gA)$ and $\Delta(\gA)$ is the probability simplex, $\pi_h (a|s)$ gives the probability of selecting action $a$ on state $s$ in time step $h$, for $h \in [H]$. 

The policy value is defined as the cumulative rewards over $H$ time steps:
\begin{align*}
    V(\pi) := \expect \ls \sum_{t=1}^{H} r(s_t, a_t) \mid s_0 \sim p_0(\cdot), a_t \sim \pi_t(\cdot|s_t), s_{t+1} \sim p_t(\cdot|s_t, a_t)  \rs .
\end{align*}
Again, we can define the non-stationary state-action distribution $\dpi_t$:
\begin{align*}
    \dpi_t(s, a) := \sP(s_t = s, a_t=a),
\end{align*}
which characterizes the probability of visiting the state-action pair $(s, a)$ in time step $t$.

\subsection{Reduction from AIL to BC}
\label{appendix:reduction_from_ail_to_bc}

\begin{thm} \label{theorem:episodic_mdp}
For episodic MDP, consider the following optimization problem:
\begin{align*}
   \min_{\pi} \sum_{t=1}^{H} \sum_{(s, a) \in \gS \times \gA} \, \, &\labs \dpi_t(s, a) - \widehat{d^{\expert}_t}(s, a) \rabs, \\
    \text{such that} \,\, & \pi_t(a|s) = 1/|\gA|, \forall s, t \text{ with } \widehat{d^{\expert}_t}(s) = 0,
\end{align*}
Assume that there is only one expert trajectory. Then, we have that the BC's policy is the globally optimal solution.
\end{thm}

\begin{proof}
To facilitate later analysis, we will use $a^{\expert}$ to denote the expert action on a specific state $s$ (recall that we assume the expert policy is deterministic). Without loss of generality, let $\widetilde{s}$ be visited state occurred in the single expert trajectory.

We want to mimic the classical dynamic programming proof as in \citep{bertsekas2012dynamic}. Specifically, we aim to prove that the BC's policy is optimal in a backward way. That is, we will use the induction proof. To this end, we define the cost function in time step $h$ as 
\begin{align*}
   \text{Loss}_h =  \sum_{(s, a) \in \gS \times \gA} \labs \dpi_h(s, a) - \widehat{d^{\expert}_h}(s, a) \rabs.
\end{align*}
Then, we can define the cost-to-go function:
\begin{align*}
    \ell_{h} = \sum_{t=h}^{H} \sum_{(s, a) \in \gS \times \gA} \labs \dpi_t(s, a) - \widehat{d^{\expert}_t}(s, a) \rabs.
\end{align*}
For the base case where time step $h = H$, we have that 
\begin{align*}
    \ell_{H} &= \sum_{(s, a)} \labs \dpi_H(s, a) - \widehat{d^{\expert}_H}(s, a) \rabs \\
    &= \sum_{a} \labs d^{\pi}_{H}(\widetilde{s}, a) - \widehat{d^{\expert}_H}(\widetilde{s}, a) \rabs + \sum_{s \ne \widetilde{s}} \sum_{a} \labs d^{\pi}_H(s, a) -  \widehat{d^{\expert}_H}(s, a) \rabs  \\
    &=  \labs d^{\pi}_{H}(\widetilde{s}, a^{\expert}) - 1 \rabs + \sum_{a \ne a^{\expert}}  \labs d^{\pi}(\widetilde{s}, a^{\expert}) - 0 \rabs  + \sum_{s \ne \widetilde{s}} \sum_{a} \labs d^{\pi}_H(s, a) - 0 \rabs \\
    &= \labs d^{\pi}_H(\widetilde{s}) \pi_{H}(a^{\expert}| \widetilde{s}) - 1 \rabs + d^{\pi}_H(\widetilde{s}) ( 1 - \pi_H(a^{\expert} | \widetilde{s})) + \sum_{s \ne \widetilde{s}} \sum_{a} d^{\pi}_H(s) \frac{1}{|\gA|} \\
    &= 1 + d^{\pi}_H(\widetilde{s}) - 2 d^{\pi}_H(\widetilde{s}) \pi_{H}(a^{\expert}|\widetilde{s})  + \sum_{s \ne \widetilde{s}} d^{\pi}_H(s) \\
    &= 1 + d^{\pi}_H(\widetilde{s}) - 2 d^{\pi}_H(\widetilde{s}) \pi_{H}(a^{\expert}|\widetilde{s})  + (1 - d^{\pi}_H(\widetilde{s})) \\
    &= 2 \lp 1 - d^{\pi}_H(\widetilde{s}) \pi_H(a^{\expert} | \widetilde{s}) \rp,
\end{align*}
which has a globally optimal solution at $\pi_H(a^{\expert}| \widetilde{s}) = 1$. This proves the base case. 

Next, for the induction step, assume we have that 
\begin{align*}
    (\pi_{h+1}(a^{\expert} | \widetilde{s}) = 1,  \pi_{h+2}(a^{\expert}|\widetilde{s}) = 1, \cdots,  \pi_{H}(a^{\expert}|\widetilde{s}) = 1) = \argmin_{\pi_{h+1}, \pi_{h+2}, \cdots, \pi_{H} } \ell_{h+1}(\pi_{h+1}, \pi_{h+2}, \cdots, \pi_{H}),
\end{align*}
where the left hand side is the \emph{unique} globally optimal solution. We want to prove that \begin{align*}
    (\pi_{h}(a^{\expert}|\widetilde{s}) = 1,  \pi_{h+1}(a^{\expert} | \widetilde{s}) = 1,   \cdots,  \pi_{H}(a^{\expert}|\widetilde{s}) = 1) = \argmin_{\pi_h, \pi_{h+1},  \cdots, \pi_{H} } \ell_{h}(\pi_h, \pi_{h+1}, \cdots, \pi_{H}) 
\end{align*}
where the left hand side is the \emph{unique} globally optimal solution.

For time step $h$, we have that 
\begin{align*}
    \text{Loss}_h  &= \sum_{(s, a)} \labs \dpi_h(s, a) - \widehat{d^{\expert}_h}(s, a) \rabs \\
    &= 2( 1 - d^{\pi}_h(\widetilde{s}) \pi_h(a^{\expert}|\widetilde{s})).
\end{align*}
For time step $h+ 1 \leq h^\prime \leq H$, we have that 
\begin{align*}
    \text{Loss}_{h^\prime}  &= \sum_{(s, a)} \labs \dpi_{h^\prime}(s, a) - \widehat{d^{\expert}_{h^\prime}}(s, a) \rabs \\
    &= 2( 1 - d^{\pi}_{h^\prime}(\widetilde{s}) \pi_{h^\prime}(a^{\expert} | \widetilde{s})) \\
    &= 2( 1 - d^{\pi}_{h^\prime}(\widetilde{s})),
\end{align*}
where the last step follows our assumption. We have the following decomposition for $d^{\pi}_{h^\prime}(\widetilde{s})$, 
\begin{align*}
    d^{\pi}_{h^\prime}(\widetilde{s}) &= \sum_{(s, a)} p_{h^\prime - 1}(\widetilde{s}|s, a) d_{h^\prime -1}^{\pi}(s, a) \\
    &= p_{h^\prime - 1}(\widetilde{s}|\widetilde{s}, a^{\expert}) d^{\pi}_{h^\prime - 1}(\widetilde{s}, a^{\expert}) +  \sum_{a \ne a^{\expert}} p_{h^\prime - 1}(\widetilde{s} | \widetilde{s}, a) d_{h^\prime - 1}^{\pi}(\widetilde{s}, a) + \sum_{s \ne \widetilde{s}} \sum_{a} p_{h^\prime - 1}(\widetilde{s}|s, a) d^{\pi}_{h^\prime -1} (s, a) \\
    &= p_{h^\prime -1}(\widetilde{s} | \widetilde{s}, a^{\expert}) d^{\pi}_{h^\prime -1}(\widetilde{s})  \pi_{h^\prime-1}(a^{\expert} | \widetilde{s}) + \sum_{a \ne a^{\expert}}p_{h^\prime -1}(\widetilde{s} | \widetilde{s}, a) d_{h^\prime -1}(\widetilde{s}) \pi_{h^\prime -1}(a| \widetilde{s}) \\
    &\quad + \sum_{s \ne \widetilde{s}} \sum_{a} p_{h^\prime - 1}(\widetilde{s}|s, a) d^{\pi}_{h^\prime -1} (s) \frac{1}{|\gA|} \\
    &= p_{h^\prime -1 } (\widetilde{s}|\widetilde{s}, a^{\expert}) d^{\pi}_{h^\prime -1}(\widetilde{s}) + \sum_{s \ne \widetilde{s}} \sum_{a} p_{h^\prime - 1}(\widetilde{s}|s, a) d^{\pi}_{h^\prime -1} (s) \frac{1}{|\gA|},
\end{align*}
where the last equation again follows our assumption.

Finally, we should have that\footnote{We have four types of transition flows: [1] $(\widetilde{s}, a^{\expert}) \rar (\widetilde{s}, a^{\expert}) \rar \cdot \rar (\widetilde{s}, a^{\expert}) \rar \widetilde{s}$; [2] $(\widetilde{s}, a) \rar (\widetilde{s}, a^{\expert}) \rar \cdots \rar (\widetilde{s}, a^{\expert}) \rar \widetilde{s}$; [3] $(\widetilde{s}, a^{\expert}) \rar (s, a) \rar \cdots \rar (s, a) \rar \widetilde{s}$; [4] $(\widetilde{s}, a) \rar (s, a) \rar \cdots \rar (s, a) \rar \widetilde{s}$. The first two terms arise in $(a)$ and the last two terms arise in $(b)$. } $\ell_h(\pi_h) = (a) + (b) + \text{constant} $, where $\text{constant}$ is unrelated to $\pi_h(\cdot| \widetilde{s})$ and 
\begin{align*}
    &(a) = -\prod_{\ell = h + 1}^{h^\prime -1 } p_{\ell}(\widetilde{s}|\widetilde{s}, a^{\expert})  \ls p_{h}(\widetilde{s}|\widetilde{s}, a^{\expert})  \pi_h(a^{\expert} | \widetilde{s}) d^{\pi}_h(\widetilde{s}) + \sum_{a \ne a^{\expert}} p_{h}(\widetilde{s}| \widetilde{s}, a) \pi_{h}(a| \widetilde{s}) d^{\pi}_h(\widetilde{s}) \rs - 2d^{\pi}_h(\widetilde{s}) \pi_h(a^{\expert}|\widetilde{s}), \\
    &(b) =  -\sum_{s \ne \widetilde{s}} \sum_{a} \frac{1}{|\gA|}  p_{h^\prime - 1}(\widetilde{s}| s, a) \bigg[ \sP(s_{h^\prime - 1} = s|s_h = \widetilde{s}, a_h = a^{\expert}) \pi_{h} (a^{\expert} |\widetilde{s}) d^{\pi}_h(\widetilde{s}) \\
    &\qquad\qquad\qquad\qquad\qquad\qquad + \sum_{a \ne a^{\expert }} \sP(s_{h^\prime - 1} = s | s_h = \widetilde{s}, a_h = a) \pi_h(a|\widetilde{s}) d^{\pi}_h(\widetilde{s}) \bigg].
\end{align*}
Let us compare the coefficient for $\pi_h(a^{\expert} | \widetilde{s})$ and $\pi_h(a|\widetilde{s})$ with $a \ne a^{\expert}$:
\begin{align*}
    c^{\expert} &= -d^{\pi}_h(\widetilde{s}) \lb \underbrace{\prod_{\ell = h + 1}^{h^\prime -1 } p_{\ell }(\widetilde{s}|\widetilde{s}, a^{\expert}) p_{h}(\widetilde{s}|\widetilde{s}, a^{\expert})}_{ \in (0, 1]} + \underbrace{\sum_{s \ne \widetilde{s}} \sum_{a} \frac{1}{|\gA|} p_{h^\prime - 1}(\widetilde{s}| s, a)  \sP(s_{h^\prime - 1} = s|s_h = \widetilde{s}, a_h = a^{\expert})}_{\in [0, 1)} + 2 \rb, \\
    c^{a} &= -d^{\pi}_h(\widetilde{s}) \lb  \underbrace{\prod_{\ell = h + 1}^{h^\prime -1 } p_{\ell}(\widetilde{s}|\widetilde{s}, a^{\expert}) p_{h}(\widetilde{s}|\widetilde{s}, a)}_{\in [0, 1]} + \underbrace{\sum_{s \ne \widetilde{s}} \sum_{a} \frac{1}{|\gA|}  p_{h^\prime - 1}(\widetilde{s}| s, a) \sP(s_{h^\prime - 1} = s | s_h = \widetilde{s}, a_h = a)}_{\in [0, 1]} \rb.
\end{align*}
Hence, $c^{\expert} < c^{a}$ and we know that $a^{\expert}$ is the optimal action in time step $h$. This proves the induction case. 

\end{proof}
